# Supplementary material for: LTGC: Long-tail Recognition via Leveraging LLMs-driven Generated Content
Source: arXiv:2403.05854 source file (2024-05-26)
Supplement: Supplementary file 1 [file X_suppl.tex]

\clearpage
\setcounter{page}{1}
\setcounter{table}{0}   %从0开始编号，显示出来表会A1开始编号
\setcounter{figure}{0}
\setcounter{section}{0}
\setcounter{equation}{0}

\maketitlesupplementary

\section{Experiments Details}
\subsection{Dataset}
We conduct the experiments on three popular long-tailed benchmarks, including ImageNet-LT \cite{liu2019large}, Places-LT \cite{liu2019large}, and iNaturalist 2018 \cite{DBLP:journals/corr/HornASSAPB17}.  We present these datasets in detail below.
% CIFAR-100-LT \cite{krizhevsky2009cifar}

\noindent\textbf{ImageNet-LT.} The ImageNet-LT \cite{liu2019large} is the long-tailed version of the dataset ImageNet-2012 \cite{imagenet}. Overall, ImageNet-LT has 115.8K images from 1000 categories with an imbalanced factor $\beta = 1280/5$. 

\noindent\textbf{Places-LT} is a long-tailed version of the large-scale scene classification dataset Places \cite{zhou2017places}. It consists of 62.5K images from 365 categories with class cardinality ranging from 5 to 4,980.

\noindent\textbf{iNaturalist 2018.} The iNaturalist 2018 \cite{DBLP:journals/corr/HornASSAPB17} is a large-scale dataset for long-tailed visual recognition rooted in real-world scenarios and exhibits a highly imbalanced distribution. It encompasses 437.5K training images and 24.4K validation images spread across 8142 categories. The dataset's fine-grained nature further intensifies its complexity.

\subsection{More Results on ImageNet-LT and Place-LT}
As shown in Tab. \ref{tab:imagenetlt} and Tab. \ref{tab:placeslt}, we present additional experimental results of our proposed LTGC on ImageNet-LT and Place-LT datasets, including results on the 'Many' and 'Medium' split sets.

\begin{table}[ht]
\footnotesize
\centering
\caption{Comparison with SOTA methods on ImageNet-LT.}
\label{tab:imagenetlt}
\begin{tabular}{c|cccc}
\hline
                        Method       &Many   &Medium     &Few &All                           \\ \hline \hline
                        CLIP Zero \cite{tian2022vlltr}         &60.8	&59.3	&58.6 &59.8        \\
                        CLIP Finetune \cite{tian2022vlltr}  &74.4	&56.9	&34.5 &60.5 	   \\  \hline
                        VL-LTR \cite{tian2022vlltr}       &77.8	&67.0	&50.8 &70.1 	    \\ \hline
                        LTGC(Ours) &\textbf{83.0}	&\textbf{79.8}	&\textbf{70.5} &\textbf{80.6}         \\
                        \hline

\end{tabular}
\vspace{-10px}
\end{table} % tab:imagenetlt

\begin{table}[ht]
\footnotesize
\centering
\caption{Comparison with SOTA methods on Places-LT.}
\label{tab:placeslt}
\begin{tabular}{c|cccc}
\hline
                        Method       &Many   &Medium     &Few &All                           \\ \hline \hline
                        CLIP Zero \cite{tian2022vlltr}         &37.5	&37.5	&40.1 &38.0     \\
                        CLIP Finetune \cite{tian2022vlltr}  &50.8	&38.6	&22.7 &39.7	   \\  \hline
                        VL-LTR \cite{tian2022vlltr}       &54.2	&48.5	&42.0 &50.1	   \\ 
                        RAC \cite{RAC}           &48.7	&48.3	&41.8 &47.2	   \\
                        LPT \cite{dong2022lpt}   &49.3	&52.3   &46.9 &50.1   \\  \hline
                        LTGC(Ours)   &\textbf{55.8}	&\textbf{54.2}	&\textbf{52.1} &\textbf{54.1}      \\
                        \hline

\end{tabular}
\vspace{-5px}
\end{table} % tab:placeslt

\subsection{Prompts for LMMs comparison.} 
For the experiments on LMMs (Sec. \ref{exp:lmms}), it's worth noting that providing a labels list significantly improves the model's performance compared to querying without a list (i.e., directly asking 'What species is in the image?'). The labels list provides prior information to the model, helping it narrow down the decision space within its extensive knowledge base. Therefore, on ImageNet-LT, we used the query template {\fontfamily{qcr}\selectfont'Please classify this image. Choose from the following classes: Class 1, Class 2, ..., Class Y.'}.

However, it is essential to note that the iNaturalist 2018 dataset encompasses a substantial number of classes, totaling 8,141, which is approximately 184 KB of text. Currently, no LLMs (including the most advanced GPT-4) are capable of processing such a lengthy input. Inputting all categories at once would lead to an error due to the limitations in text length. Dividing the categories into multiple inputs would cause the model to forget previous categories, leading to inaccurate judgments based on the most recent inputs.
Therefore, for the iNaturalist dataset, we adopted the query template {\fontfamily{qcr}\selectfont'What species is in the image?'} for testing purposes. We then reviewed the entire response, considering the LLMs' classification as correct if it included any vocabulary matching the Ground Truth class, and as incorrect otherwise.

\begin{table}[ht]
\centering
\caption{Effectiveness of the Self-reflection module. \textbf{NC}: Number-checking. \textbf{RC}: Repetition-checking.}
\label{tab:checking}
\begin{tabular}{c|cc|c}
\hline
                         Dataset           & \text{NC} & \text{RC}  & Top-1 Accuracy            \\ \hline
                         \multirow{4}{*}{ImageNet-LT}
                                           &{-}	&{-}	&60.5	   \\
                                           &{\checkmark}	&{-}	&71.7	  \\ 
                                           &{-} &{\checkmark}		&73.2	  \\ 
                                           &{\checkmark} &{\checkmark}	&80.6	  \\  \hline
                         \multirow{4}{*}{iNaturalist 2018}
                                           &{-} &{-}		&71.6	   \\
                                           &{\checkmark} &{-}		&78.4	  \\ 
                                           &{-} &{\checkmark}   	&71.8	  \\ 
                                           &{\checkmark} &{\checkmark} 	&82.5	  \\  \hline
\end{tabular}
\vspace{-0.05in}
\end{table} % tab:checking

\section{Additional Ablation Studies}
Here, we conduct additional ablation experiments. Unless otherwise noted, we report the top-1 accuracy averaged over three runs on the ImageNet-LT evaluation protocol.

\textbf{Effectiveness of the Self-reflection module.} 
The self-reflection module consists of two elements: a number check for images and a repetition check. We separately investigated these two checks, and the results are shown in Tab. \ref{tab:checking}.
When only performing the quality check, LLMs generate highly repetitive descriptions, leading to a decrease in textual diversity and, consequently, a decline in image diversity.
When only performing the repetitiveness check, the LLMs are posed the two questions mentioned in Section \ref{subsecgeneration} only once. This results in a limited number of generated samples, thereby leading to limited performance gains.
As shown in Tab. \ref{tab:checking}, our proposed method incorporates both checks and consistently outperforms all variants. This attests to (1) the effectiveness of the repetitiveness design, enabling LLMs to generate comprehensive text descriptions, and (2) the efficacy of the self-reflection design, allowing LLMs to increase the number of samples and simulate a more balanced set of classes.

\textbf{Impact of using different versions of ChatGPT of LLM.} Besides, we also test using different versions of ChatGPT with different capabilities, including GPT 3.0, GPT-3.5 Turbo 16K, and the latest GPT-4 Turbo 128K. As shown in Tab. \ref{tab:gpt-sp}, our framework with different versions of GPT used can achieve different results. This shows that the performance of our framework is affected by the version of ChatGPT.

\begin{table}[ht]
\centering
\caption{Evaluation on using different versions of ChatGPT.}
\label{tab:gpt-sp}
\begin{tabular}{c|c|c}
\hline
                         Version                 &ImageNet-LT   &iNaturalist            \\ \hline
                         GPT 3.0               &72.0		    &74.1	   \\
                         GPT 3.5               &76.9     	&79.3	  \\ 
                         GPT 4.0               &80.6		    &82.5	  \\  \hline
\end{tabular}
\vspace{-0.05in}
\end{table} % tab:gpt-sp
 
\textbf{The effectiveness of different maximum image numbers for LLM's self-reflection module.}
In our framework, the maximum number of generated and original images for each class $y$, denoted as $K_y$. For LLM's self-reflection module, the $K_y$ is set to 100 for iNaturalist 2018, 300 for ImageNet-LT, and 800 for Place-LT, respectively.
We explore alternative caps for the maximum image number and show the findings in Fig. \ref{fig:supp-maximg}.
The results indicate that for each dataset when the cap is set below 100, 300, and 800, respectively, there's a noticeable improvement in our framework’s performance as the limit on generative images increases.
This might be because, by setting the maximum number of images to be a larger number, LLM can better cover the diverse distinctive features and backgrounds (scenes).
Moreover, it's observed that increasing the maximum image number beyond 100, 300, and 800 does not lead to further improvements in performance.
However, surpassing these maximum numbers of 100, 300, and 800 doesn't yield further performance gains. Therefore, balancing performance and efficiency, we determined these respective limits as the optimal settings for our framework.

\begin{figure}[ht]
  \centering
    % \fbox{\rule{0pt}{2in} \rule{.9\linewidth}{0pt}}
    \includegraphics[width=0.95\linewidth]{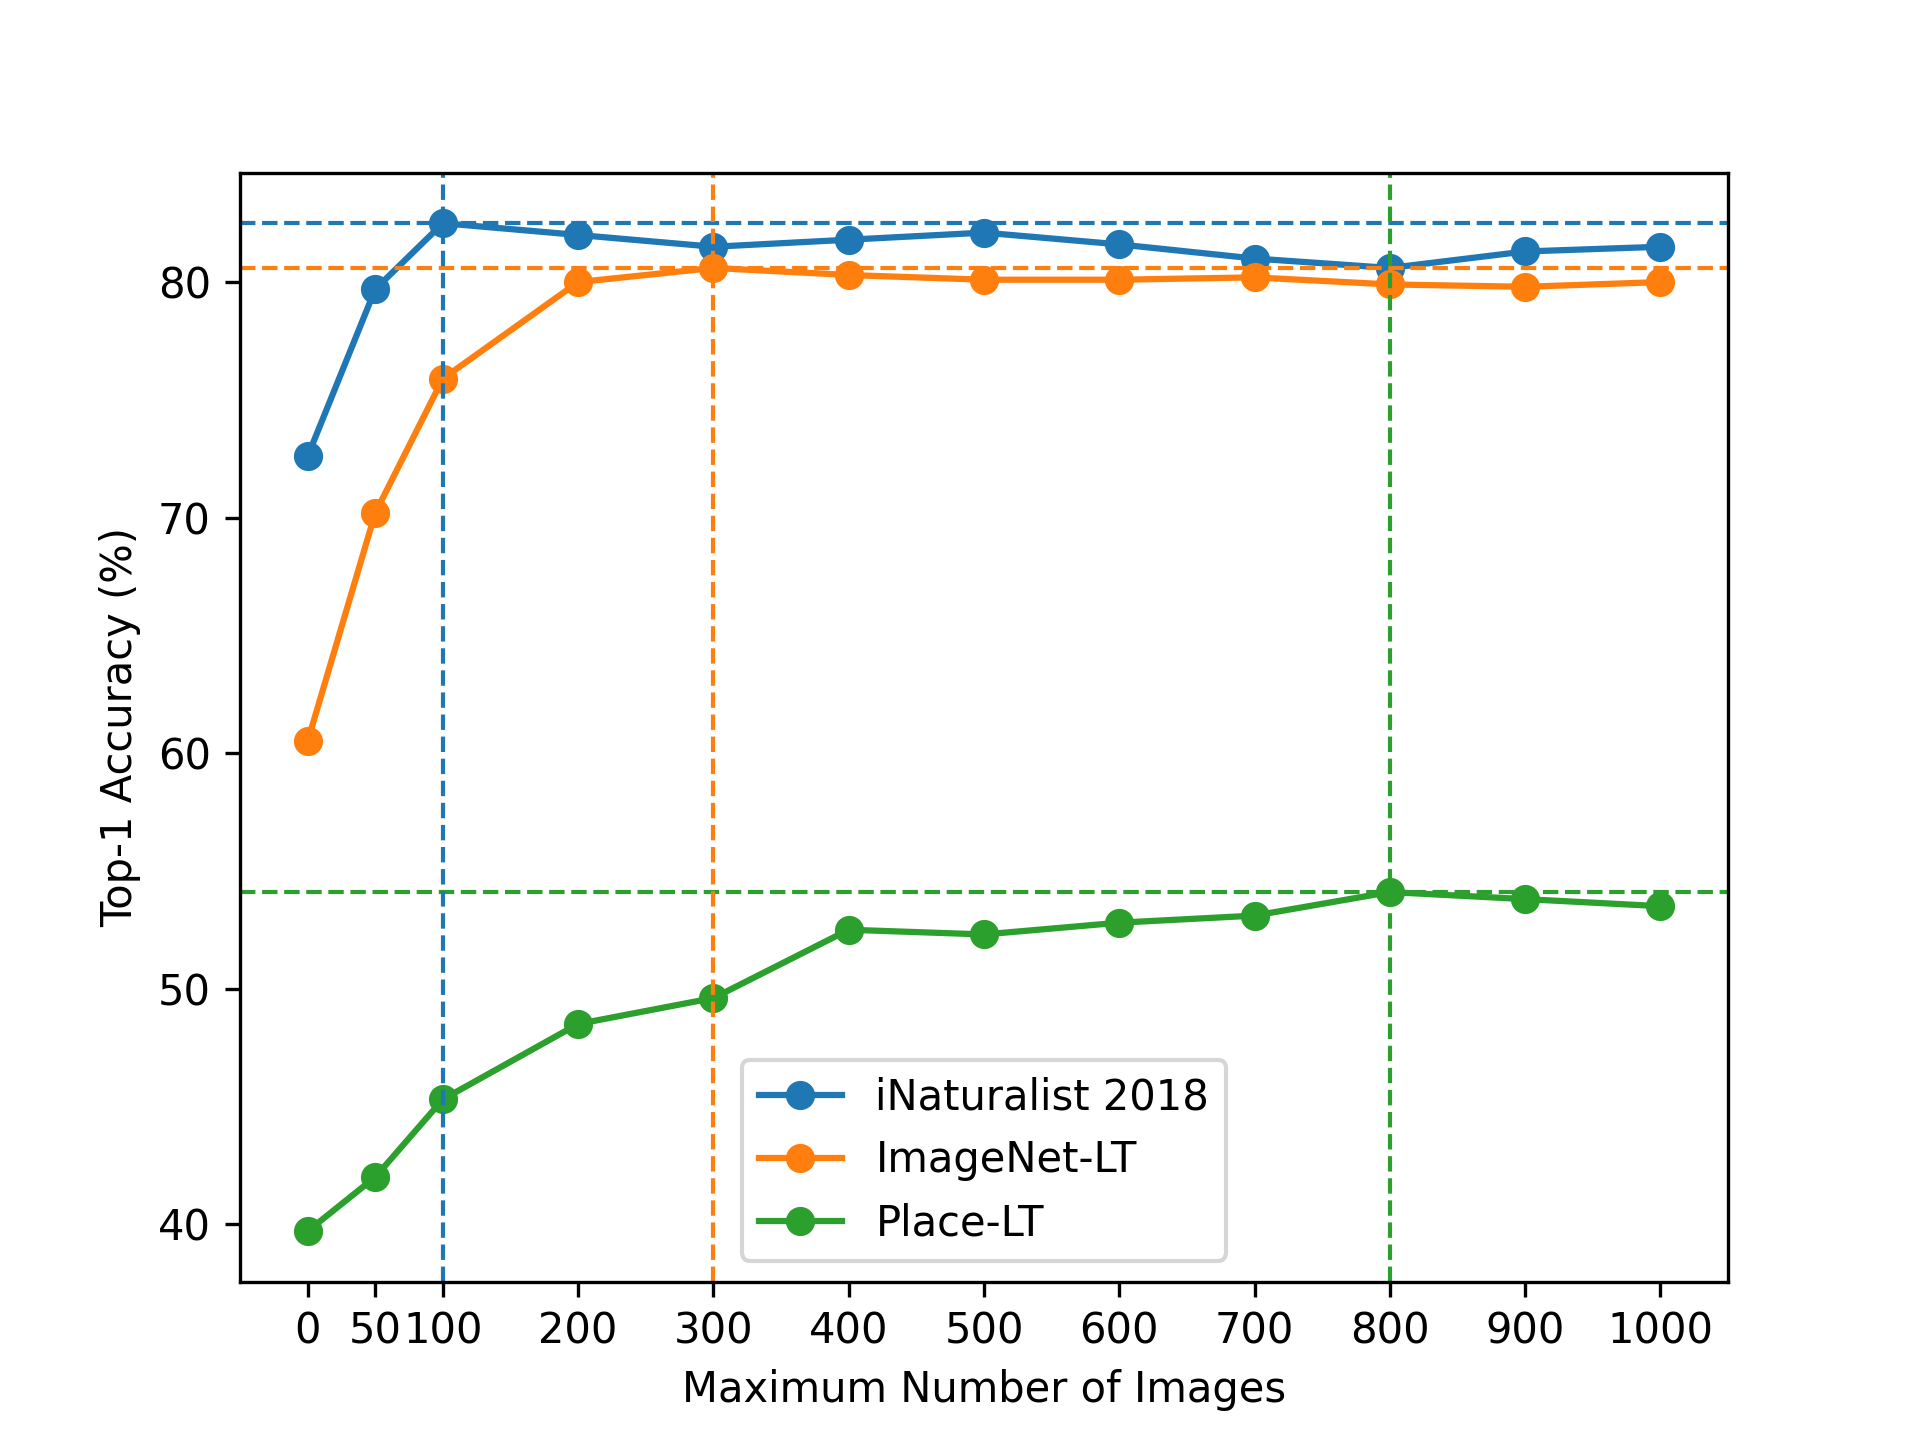}
    \caption{\textbf{The effectiveness of different maximum image numbers for LLM's self-reflection module.}}
    \label{fig:supp-maximg}
\vspace{-10px}
\end{figure} % fig:maximg

\textbf{Impact of the maximum number of cycle times for iterative evaluation module.} In our framework's iterative evaluation module, we initially cap the cycle count at three. To explore the impact of varying this limit, we experimented with different maximum cycle thresholds and presented the outcomes in Table \ref{tab:time-sp}. The results indicate an enhancement in our framework's performance as we expand the maximum cycle count for iterative evaluation. This improvement is likely due to the more thorough refinement of generated images achieved with a higher cycle limit. However, the gains in performance diminish when the cycle count exceeds three, leading us to establish three as the optimal maximum for the iterative evaluation module.

\begin{table}[ht]
\centering
\caption{Evaluation on the maximum number of cycle times for iterative evaluation.}
\label{tab:time-sp}
\begin{tabular}{c|c}
\hline
                         Maximum number of cycle time               &ImageNet-LT     \\ \hline
                         1                &71.5     		  \\ 
                         2                &78.1		   	  \\ 
                         3                &80.6		   \\ 
                         4                &79.9		   \\ 
                         \hline 
\end{tabular}
\vspace{-0.05in}
\end{table} % tab:time-sp

\textbf{Check the reasonability of the generated descriptions.} In our framework, we use ChatGPT to generate text descriptions for the evaluated classes, and we further design a iterative evaluation module in which we guide ChatGPT to modify its generated descriptions. Here, we perform a check w.r.t. the reasonability of the generated descriptions before and after passing into the iterative evaluation module. Specifically, we find that, before passing into the iterative evaluation module, 4\% of descriptions are checked to be unreasonable, but 0.2\% of the descriptions output by the module is checked to be unreasonable. This shows that ChatGPT has small probability of generating unreasonable descriptions, while our iterative evaluation module can further mitigate this problem. The above check is done by inviting 3 volunteers and passing the same 1000 descriptions to them. The 3 volunteers first make decisions independently and then discuss disagreed decisions.

\begin{figure*}[h]
  \centering
  \begin{subfigure}{0.9\linewidth}
    % \fbox{\rule{0pt}{2in} \rule{.9\linewidth}{0pt}}
    \includegraphics[width=1.0\linewidth]{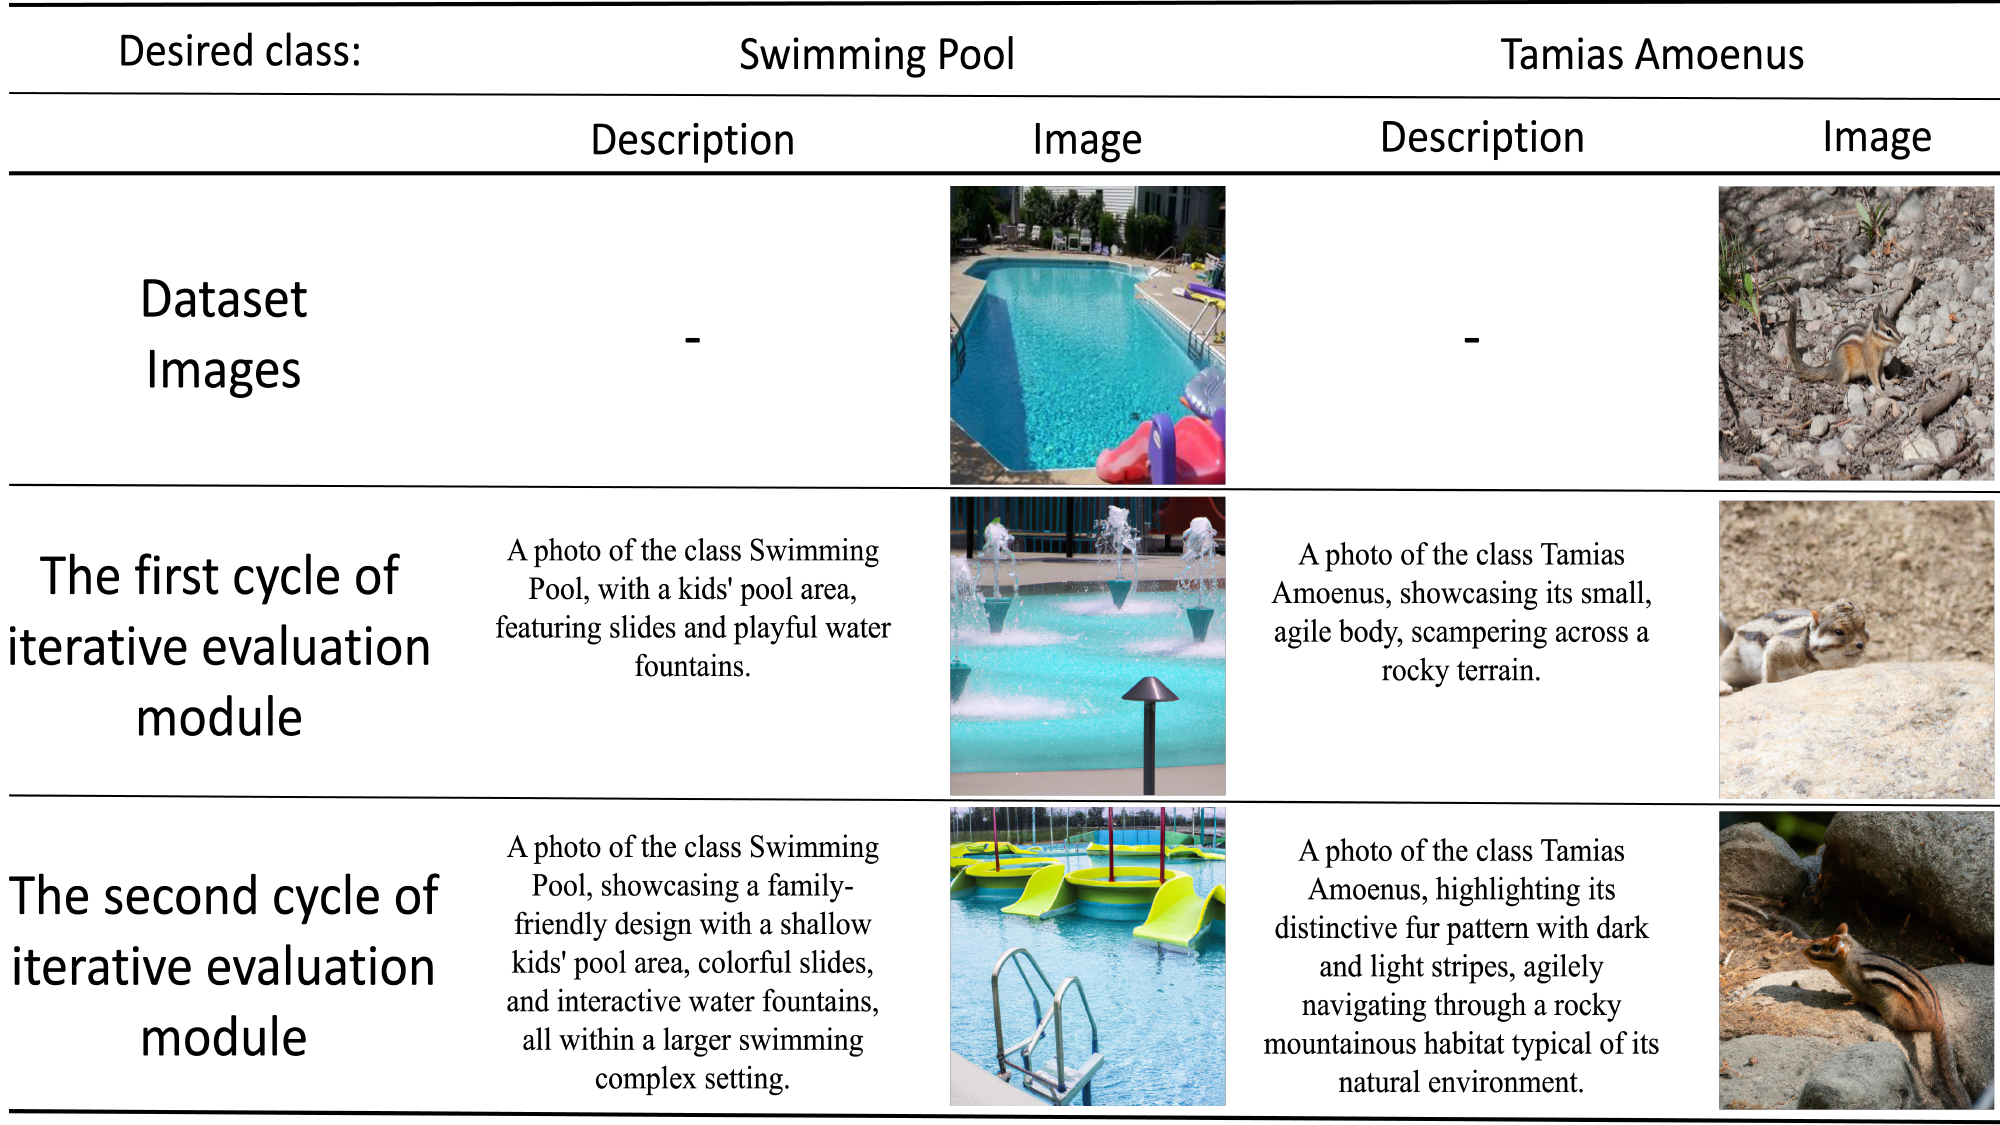}
    %\captionsetup{font=Medium}
    \caption{  }
    \label{fig:2cycle}
    \vspace{10px}
  \end{subfigure}
  \hfill
  \begin{subfigure}{0.9\linewidth}
    % \fbox{\rule{0pt}{2in} \rule{.9\linewidth}{0pt}}
    \includegraphics[width=1.0\linewidth]{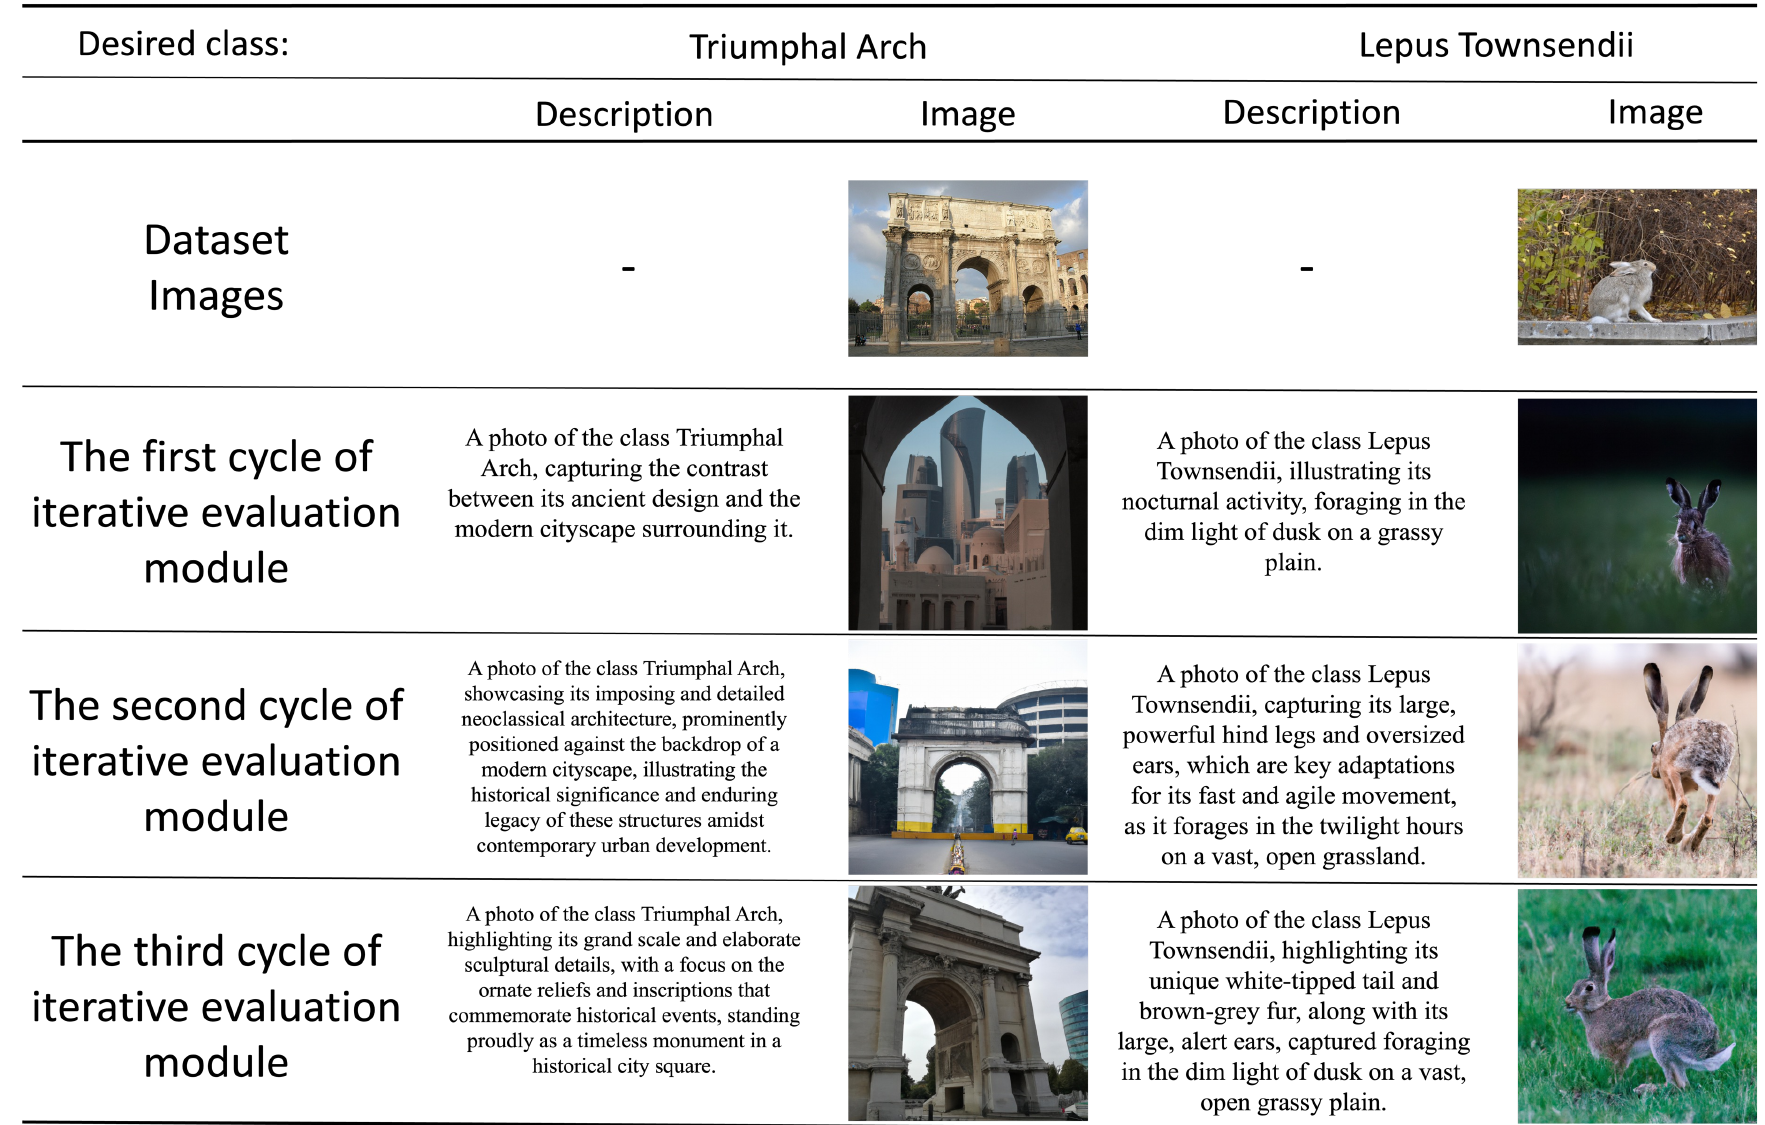}
    %\captionsetup{font=Medium}
    \caption{  }
    \label{fig:3cycle}
  \end{subfigure}
  \caption{Visualization about the iterative evaluation module. The images in (a) do not align most closely with their intended classes until the third cycle, whereas the images in (b) achieve their closest alignment with the intended classes in the second cycle. 
  The classes of \textit{Tamias Amoenus} and \textit{Lepus Townsendii} are derived from the iNaturalist dataset, while \textit{Swimming Pool} and \textit{Triumphal Arch} are from the Place-LT and ImageNet-LT datasets, respectively.}
  \label{fig:supp-cycle}
\end{figure*} % cycle_vis

\textbf{Preparation time.} 
In our framework, before entering the fine-tuning process, we first prepare the generated images by extending the descriptions of tail classes and then generate diverse images for each class, filtering and regenerating the low-quality images. We here report the preparation time of our framework. For generating images, the speed of image generation is limited by DALL-E's API, about 50 images/minute \cite{ramesh2021zero}. For generating descriptions, the speed is about 300 items/minute. Note that the entire preparation process of our framework can be automated by a script with multi-threaded accelerated generation.

\textbf{The effectiveness of fine-tuning with LoRA.} In the fine-tuning process, we fine-tune the visual encoder of the CLIP model using Low-Rank Adaptation (LoRA) \cite{hu2021lora}, LoRA layers are typically added to the Transformer layers of the CLIP model. The main idea of LoRA is to make low-rank modifications to existing weight matrices, rather than updating all parameters directly. This method is often used in large-scale models to achieve effective and parameter-efficient fine-tuning.

Each Transformer layer in the CLIP model consists of two main components: the Multi-Head Self-Attention and the Feedforward Neural Network. LoRA can be applied to the weight matrices of both these components.

Specifically, in the Multi-Head Self-Attention, LoRA can be applied to the Query, Key, and Value matrices. For the Feedforward Network, LoRA can be integrated into the first linear transformation, which is right before the ReLU activation function. 

Moreover, other competitive methods of parameter fine-tuning have emerged in recent years, such as VQT \cite{tu2023visualVQT}. In Tab. \ref{tab:lora} we compare LoRA with other fine-tuning methods such as Linear-probing \cite{radford2021clip} and VQT \cite{tu2023visualVQT}. We observe that LoRA outperforms other fine-tuning methods, demonstrating the effectiveness of our fine-tuning with LoRA

\begin{table}[ht]
\centering
\footnotesize
\caption{The effectiveness of fine-tuning with LoRA.}
\label{tab:lora}
\begin{tabular}{c|c|c}
\hline
                         Method                 &ImageNet-LT   &iNaturalist            \\ \hline
                         Linear-probing \cite{radford2021clip}      &71.4		&66.3	   \\
                         VQT \cite{tu2023visualVQT} &77.3     	&78.1	  \\ 
                         LoRA (Ours)              &80.6		&82.5	  \\  \hline
\end{tabular}
\vspace{-15px}
\end{table} % tab:blsmix

\begin{figure}[ht]
  \centering
    % \fbox{\rule{0pt}{2in} \rule{.9\linewidth}{0pt}}
    \includegraphics[width=0.95\linewidth]{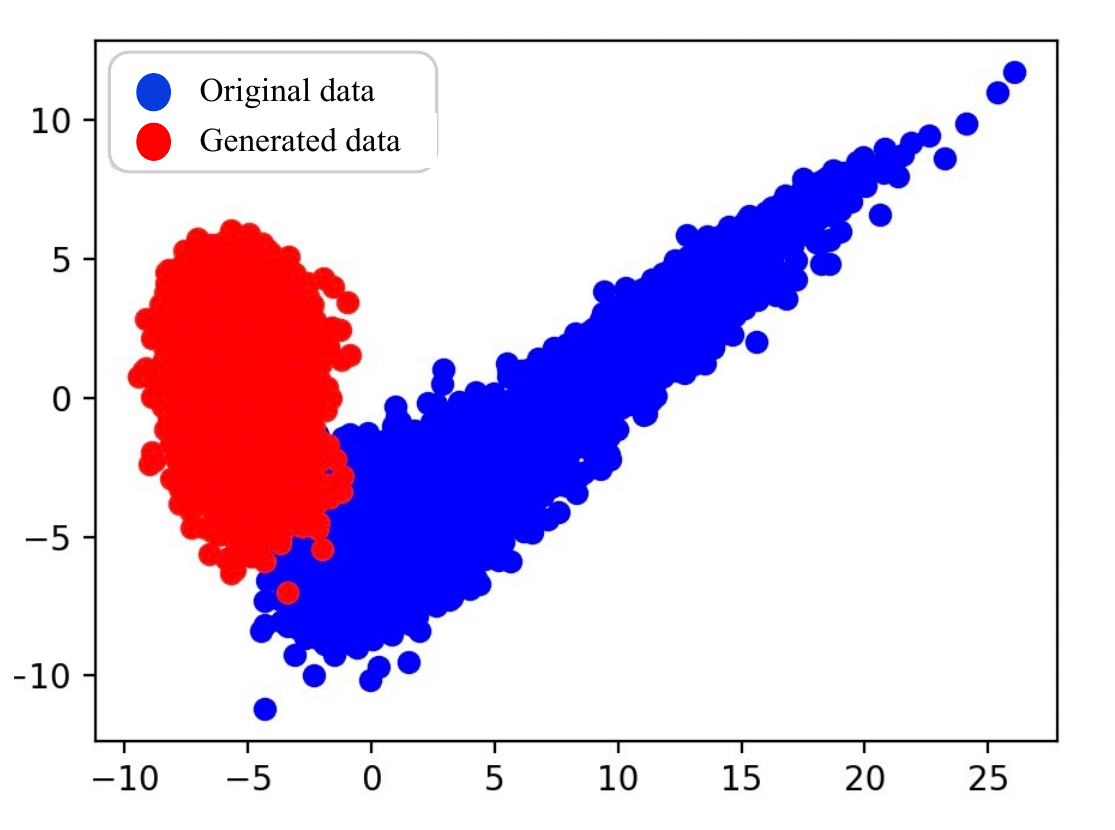}
    \caption{\textbf{Domain gap between generated images and original images.}}
    \label{fig:domaingap}
\vspace{-10px}
\end{figure} % fig:domaingap

\section{Additional Visualizations}

\textbf{Visualisation of the iterative evaluation module.} 
In this work, we propose an iterative evaluation module for our framework. This module aims to enhance the quality of generated images, particularly those that are not highly accurate. Fig \ref{fig:supp-cycle} illustrates the refinement process carried out by our iterative evaluation module. As depicted, this module effectively improves images that initially do not align well with their intended classes, ensuring they more accurately represent these classes. This highlights the efficiency and utility of our iterative evaluation module in image refinement.

\textbf{Domain gap between generated images and original images.}
Some previous methods have shown that there is a domain gap \cite{trabucco2023effective} between the generated data and the original data, to better illustrate the domain gap we visualize the t-SNE \cite{van2008visualizing} results for the part of the original data and the part of generated data. In Fig. \ref{fig:domaingap}, we observe that there is a domain gap between the generated data and the original data. This motivated us to propose the BalanceMix method and significantly helped the model fine-tuning to improve the recognition results.

\section{Licenses}

\textbf{Large model licenses.} We use ChatGPT and DALL-E by following the terms of using the services of OpenAI. We use CLIP by following the MIT License.
